# Supplementary material for: Evaluating Computational Language Models with Scaling Properties of Natural Language
Source: arXiv:1906.09379 source file (2019-06-22)
Supplement: Supplementary file 1 [file appendix0.tex]

\newpage
\onecolumn
\section*{Appendix A: The property of negative log-likelihood of PCFG}
We argued that the negative log-likelihood of PCFG cannot be utilized to evaluate the quality of natural language. 
This appendix adds an evidence to strengthen our argument.
The scatter plot \figref{fig:pcfg-dist} is the negative log likelihood of PCFG for the PTB dataset, 
AWD-LSTM-Cache and fivegram shuffled PTB dataset.
The negative log likelihood of the PTB dataset is consistently lower than that of the generated text of AWD-LSTM-Cache and fivegram shuffled text.
However, the performance of PCFG as an evaluation metrics remain questionable.
The shaded area represents the upper bound and lower bound of the negative log likelihood of PCFG for the PTB dataset.
The average values of the fivegram shuffled text and the machine generated text are in the range of the bounds.
This indicates that the negative log likelihood of PCFG is not suited for the evaluation of one sentence.
The negative log-likelihood of a sentence has a strong linear correlation with its length
Further, because the large scaled parsed corpus is scarcely available other than the PTB dataset,
the application is limited to the specific dataset.

\begin{figure*}[h]
	\centering
	\includegraphics[width=10.0cm]{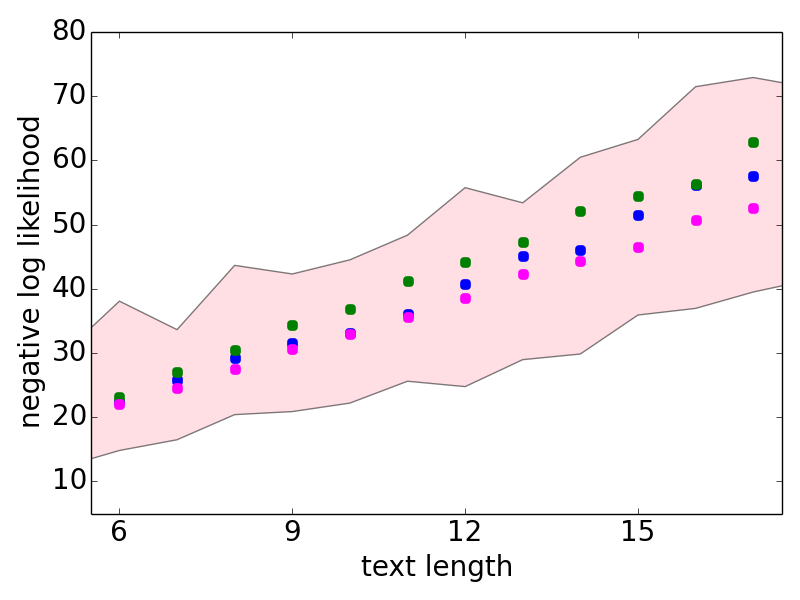}
	%\hspace*{-0.2cm}
	\caption{Sentence length versus the negative log likelihood of PCFG for the PTB dataset (pink), AWD-LSTM-Cache (blue) and fivegram shuffled PTB dataset (green). The pink shaded area represents the upper bound and and lower bound of the negative log likelihood of PCFG for the PTB dataset.}
	\label{fig:pcfg-dist}
\end{figure*}
